# Supplementary material for: Craig Interpolation for Guarded Fragments
Source: arXiv:2304.08086 source file (2023-04-17)
Supplement: Supplementary file 1 [file appendix.tex]

\documentclass[oneside, notitlepage]{book}
\usepackage{amsmath}
\usepackage{amssymb}
\usepackage{amsthm}
\usepackage{letltxmacro}
\usepackage{changepage}
\usepackage{qtree}
\usepackage[margin=.75in]{geometry}
\usepackage{enumitem}
\usepackage{mathtools}
\usepackage{tikz}
\usetikzlibrary{positioning,calc}
\setenumerate[1]{label=(\arabic*)}
\usepackage{algorithm}
\usepackage[noend]{algpseudocode}
\usepackage{hyperref}
\usepackage{xpatch}
\usepackage{upgreek}
\usepackage{bussproofs}
\usepackage{graphicx}

\makeatletter
\providecommand*{\dashV}{%
  \mathrel{%
    \mathpalette\@dashV\models
  }%
}
\newcommand*{\@dashV}[2]{%
  \reflectbox{$\m@th#1#2$}%
}
\makeatother

\hypersetup{
    colorlinks=true,
    linkcolor=magenta,
    filecolor=magenta,      
    urlcolor=magenta,
    pdftitle={Overleaf Example},
    pdfpagemode=FullScreen,
    }

\theoremstyle{definition}

\makeatletter
\newcommand*{\toccontents}{\@starttoc{toc}}
\makeatother
  
\DeclarePairedDelimiter\ceil{\lceil}{\rceil}
\DeclarePairedDelimiter\floor{\lfloor}{\rfloor}

\theoremstyle{definition}
\newtheorem{theorem}[equation]{Theorem}
\newtheorem{definition}[equation]{Definition}
\newtheorem{remark}[equation]{Remark}
\newtheorem{proposition}[equation]{Proposition}
\newtheorem{example}[equation]{Example}
\newtheorem{lemma}[equation]{Lemma}
\newtheorem{corollary}[equation]{Corollary}

%Notation
\newcommand{\Cases}{\mathbf{cases}}

\xpatchcmd{\proof}{\itshape}{\normalfont\proofnamefont}{}{}
\newcommand{\proofnamefont}{\bfseries}
\LetLtxMacro\oldproof\proof
\let\endoldproof\endproof
\renewenvironment{proof}[1][\proofname]{\begin{adjustwidth}{.3in}{.3in}\oldproof[#1]}{\endoldproof\end{adjustwidth}}


%%%%%%%%%%%%%%%%%%%%%%%%%%%%%%%%%%%%%%%%%%%%%%%%%%%%%%%%%%%%%%%
\begin{document}
\begin{flushleft}
%%%%%%%%%%%%%%%%%%%%%%%%%%%%%%%%%%%%%%%%%%%%%%%%%%%%%%%%%%%%
\section*{Appendix: Expressibility of UCQs}

\input{../appendix-text}



















\end{flushleft}

\end{document}
